# Supplementary material for: Initialization and Alignment for Adversarial Texture Optimization
Source: arXiv:2207.14289 source file (2022-07-28)
Supplement: Supplementary file 1 [file ethics.tex]

\section{Ethics Statement}\label{supp sec: ethics}

\subsection{Potential Negative Societal Impacts}

We study the problem of texture reconstruction from single-camera RGBD videos. Two potential negative impacts may occur if such technologies are not used properly:
\begin{itemize}
    \item This framework may be used to reconstruct private property without permission of the property owner, which may violate privacy;
    \item Although we only consider static scenes in this paper, the framework currently does not have a specific procedure to exclude dynamic objects,~\eg,~humans. If dynamic objects are not explicitly removed from images, the resulting texture may contain personally identifiable information,~\eg,~humans' faces, invading privacy. This potential impact can be alleviated by incorporating human detection approaches to mask out humans from each frame.  
\end{itemize}

\subsection{Ethical Conduct}

The dataset we collected contains neither personally identifiable information nor offensive content.
